# Supplementary material for: Infrared Object Detection with Ultra Small ConvNets: Is ImageNet Pretraining Still Useful?
Source: arXiv:2508.02927 ancillary file (2026-01-19)
Supplement: Supplementary file 1 [file supplementary.pdf]

# Supplementary Material for Infrared Object Detection with Ultra Small ConvNets: Is ImageNet Pretraining Still Useful?

Srikanth Muralidharan    Heitor R. Medeiros    Masih Aminbeidokhti  
Eric Granger    Marco Pedersoli  
LIVIA, Dept. of Systems Engineering, ETS Montreal, Canada  
International Laboratory on Learning Systems (ILLS)

## 1. Small Model Generation

### 1.1. Smaller variants for EfficientNet

EfficientNet-B0 comprises a stem module, seven subsequent blocks, a convolutional head, and final classification components. In this section, we describe our process of scaling down EfficientNet-B0, which contains millions of parameters, to ultra-small networks with only tens of thousands of parameters.

We adopt two protocols for constructing these compact models. First, we downscale the width and depth of EfficientNet without modifying its block semantics. In the second protocol, we alter the semantics of the EfficientNet blocks by modifying the squeeze-and-excite modules.

#### 1.1.1. Depth-Width Downscaling of EfficientNet

We downscale the width and depth of EfficientNet using its original scaling law conventions while maintaining constant input dimensions. Since our end task is object detection, we keep the input resolution unchanged to avoid degrading its performance. Specifically, EfficientNet introduces a compound scaling method that uniformly scales the network depth, width, and resolution using a set of predetermined constants [3]. We modify this compound scaling method to keep the resolution constant, while changing width and depth for our models. Our scaling operation is performed as follows:

$$\begin{aligned} \text{Depth : } d &= \alpha^\phi, \\ \text{Width : } w &= \beta^\phi, \end{aligned} \tag{1}$$

subject to the constraint:

$$\alpha \cdot \beta^2 \approx 2, \tag{2}$$

where  $\phi$  is the compound scaling coefficient that controls overall model size, and  $\alpha, \beta$  are constants determined via

grid search to balance performance and efficiency. It is important to note here that the key distinction between compound scaling used in EfficientNet and ours is the absence of resolution scaling factor  $\gamma$ . The compound scaling done this way therefore enables us to stay as close to EfficientNet’s original compound scaling as possible while retaining focus on our end task which is object detection in non-RGB visual domains. We start from EfficientNet-B0 and scale down until seven levels below it. Therefore the value  $\phi$  in our case ranges from  $-7$  to  $-1$ .

### 1.2. Smaller variants for MobileNet-V3

We start from Mobilenet-V3 small [1] and downscale upto six levels after the small model. With each downscaling, for each model, we roughly cut the number of parameters by roughly 50% compared to the model a level higher to it. We downsize both the width and the depth using the scaling framework from Mobilenet-v3. Further, for each downscaling we use same multiplier parameter for both width and depth multiplier.

## 2. Detailed tabular in-domain and out-domain results

Here we report tabular results for LLVIP, FLIR and distech datasets. LLVIP results are presented in tables 1 and 2 for EfficientNet and MobileNet model families respectively. FLIR dataset’s numbers are presented in 3 and 4. Finally, performance of models on Distech dataset are reported in tables 5 and 6 for EfficientNet and MobileNet models respectively.

## References

- [1] Andrew G Howard, Menglong Zhu, Bo Chen, Dmitry Kalenichenko, Weijun Wang, Tobias Weyand, Marco Andreetto, and Hartwig Adam. Mobilenets: Efficient convolutional neural networks for mobile vision applications. *arXiv preprint arXiv:1704.04861*, 2017. 1

| Model | Pretrained | mAP-ID            | mAP50-ID          | mAP-OOD           | mAP50-OOD         |
|-------|------------|-------------------|-------------------|-------------------|-------------------|
| B0    | True       | 0.439             | 0.848             | 0.326             | 0.666             |
| B0    | False      | 0.410             | 0.799             | 0.259             | 0.547             |
| B-1   | True       | $0.408 \pm 0.014$ | $0.795 \pm 0.024$ | $0.304 \pm 0.006$ | $0.634 \pm 0.026$ |
| B-1   | False      | $0.415 \pm 0.007$ | $0.801 \pm 0.011$ | $0.300 \pm 0.027$ | $0.607 \pm 0.054$ |
| B-2   | True       | $0.388 \pm 0.010$ | $0.777 \pm 0.015$ | $0.299 \pm 0.007$ | $0.654 \pm 0.023$ |
| B-2   | False      | $0.378 \pm 0.007$ | $0.752 \pm 0.016$ | $0.256 \pm 0.006$ | $0.548 \pm 0.019$ |
| B-3   | True       | $0.360 \pm 0.002$ | $0.742 \pm 0.003$ | $0.245 \pm 0.020$ | $0.547 \pm 0.048$ |
| B-3   | False      | $0.358 \pm 0.005$ | $0.737 \pm 0.010$ | $0.238 \pm 0.006$ | $0.531 \pm 0.009$ |
| B-4   | True       | $0.342 \pm 0.005$ | $0.751 \pm 0.012$ | $0.146 \pm 0.016$ | $0.406 \pm 0.053$ |
| B-4   | False      | $0.349 \pm 0.007$ | $0.738 \pm 0.012$ | $0.187 \pm 0.033$ | $0.442 \pm 0.084$ |
| B-5   | True       | $0.340 \pm 0.003$ | $0.750 \pm 0.005$ | $0.152 \pm 0.006$ | $0.391 \pm 0.012$ |
| B-5   | False      | $0.346 \pm 0.018$ | $0.730 \pm 0.036$ | $0.194 \pm 0.019$ | $0.448 \pm 0.045$ |
| B-6   | True       | $0.326 \pm 0.004$ | $0.726 \pm 0.010$ | $0.162 \pm 0.020$ | $0.403 \pm 0.050$ |
| B-6   | False      | $0.339 \pm 0.007$ | $0.731 \pm 0.015$ | $0.199 \pm 0.020$ | $0.490 \pm 0.056$ |
| B-7   | True       | $0.313 \pm 0.007$ | $0.710 \pm 0.012$ | $0.152 \pm 0.008$ | $0.400 \pm 0.018$ |
| B-7   | False      | $0.331 \pm 0.010$ | $0.735 \pm 0.009$ | $0.151 \pm 0.067$ | $0.365 \pm 0.147$ |

Table 1. Performance comparison on LLVIP dataset [2] with and without ImageNet pretraining at (384,384) pre-training and (384,480) fine-tuning resolution for EfficientNet family models.

| Model | Pretrained | mAP-ID            | mAP50-ID          | mAP-OOD           | mAP50-OOD         |
|-------|------------|-------------------|-------------------|-------------------|-------------------|
| S     | True       | $0.202 \pm 0.001$ | $0.463 \pm 0.002$ | $0.059 \pm 0.003$ | $0.157 \pm 0.006$ |
| S     | False      | $0.184 \pm 0.003$ | $0.416 \pm 0.002$ | $0.043 \pm 0.006$ | $0.118 \pm 0.014$ |
| S-1   | True       | $0.181 \pm 0.003$ | $0.419 \pm 0.004$ | $0.055 \pm 0.003$ | $0.155 \pm 0.014$ |
| S-1   | False      | $0.177 \pm 0.002$ | $0.404 \pm 0.007$ | $0.039 \pm 0.005$ | $0.107 \pm 0.015$ |
| S-2   | True       | $0.172 \pm 0.003$ | $0.395 \pm 0.005$ | $0.047 \pm 0.001$ | $0.127 \pm 0.002$ |
| S-2   | False      | $0.174 \pm 0.003$ | $0.393 \pm 0.006$ | $0.036 \pm 0.007$ | $0.101 \pm 0.024$ |
| S-3   | True       | $0.156 \pm 0.003$ | $0.358 \pm 0.004$ | $0.023 \pm 0.004$ | $0.067 \pm 0.009$ |
| S-3   | False      | $0.163 \pm 0.003$ | $0.373 \pm 0.008$ | $0.036 \pm 0.005$ | $0.102 \pm 0.013$ |
| S-4   | True       | $0.150 \pm 0.001$ | $0.354 \pm 0.004$ | $0.031 \pm 0.004$ | $0.090 \pm 0.012$ |
| S-4   | False      | $0.150 \pm 0.007$ | $0.348 \pm 0.014$ | $0.040 \pm 0.003$ | $0.115 \pm 0.007$ |
| S-5   | True       | $0.141 \pm 0.001$ | $0.338 \pm 0.004$ | $0.022 \pm 0.002$ | $0.067 \pm 0.007$ |
| S-5   | False      | $0.141 \pm 0.001$ | $0.322 \pm 0.004$ | $0.035 \pm 0.005$ | $0.101 \pm 0.014$ |
| S-6   | True       | $0.136 \pm 0.002$ | $0.323 \pm 0.004$ | $0.023 \pm 0.003$ | $0.069 \pm 0.005$ |
| S-6   | False      | $0.140 \pm 0.002$ | $0.330 \pm 0.005$ | $0.023 \pm 0.003$ | $0.066 \pm 0.007$ |

Table 2. Performance comparison on LLVIP dataset [2] with and without ImageNet pretraining at (384,384) pre-training and (384,480) fine-tuning resolution for MobileNet family models.

- [2] Xinyu Jia, Chuang Zhu, Minzhen Li, Wenqi Tang, and Wenli Zhou. Llvp: A visible-infrared paired dataset for low-light vision. In *Proceedings of the IEEE/CVF International Conference on Computer Vision*, pages 3496–3504, 2021. 2
- [3] Mingxing Tan and Quoc Le. Efficientnet: Rethinking model scaling for convolutional neural networks. In *International conference on machine learning*, pages 6105–6114. PMLR, 2019. 1

| Model | Pretrained | mAP-ID            | mAP50-ID          | mAP-OOD           | mAP50-OOD         |
|-------|------------|-------------------|-------------------|-------------------|-------------------|
| B-0   | True       | 0.249 $\pm$ 0.000 | 0.560 $\pm$ 0.000 | 0.122 $\pm$ 0.000 | 0.303 $\pm$ 0.000 |
| B-0   | False      | 0.256 $\pm$ 0.000 | 0.560 $\pm$ 0.000 | 0.113 $\pm$ 0.000 | 0.277 $\pm$ 0.000 |
| B-1   | True       | 0.245 $\pm$ 0.001 | 0.545 $\pm$ 0.003 | 0.096 $\pm$ 0.007 | 0.252 $\pm$ 0.023 |
| B-1   | False      | 0.239 $\pm$ 0.000 | 0.521 $\pm$ 0.002 | 0.070 $\pm$ 0.027 | 0.169 $\pm$ 0.072 |
| B-2   | True       | 0.214 $\pm$ 0.002 | 0.489 $\pm$ 0.005 | 0.076 $\pm$ 0.007 | 0.190 $\pm$ 0.013 |
| B-2   | False      | 0.203 $\pm$ 0.002 | 0.458 $\pm$ 0.006 | 0.054 $\pm$ 0.027 | 0.137 $\pm$ 0.068 |
| B-3   | True       | 0.182 $\pm$ 0.002 | 0.424 $\pm$ 0.006 | 0.044 $\pm$ 0.002 | 0.120 $\pm$ 0.006 |
| B-3   | False      | 0.181 $\pm$ 0.004 | 0.413 $\pm$ 0.012 | 0.043 $\pm$ 0.012 | 0.113 $\pm$ 0.036 |
| B-4   | True       | 0.163 $\pm$ 0.000 | 0.381 $\pm$ 0.002 | 0.032 $\pm$ 0.002 | 0.090 $\pm$ 0.004 |
| B-4   | False      | 0.161 $\pm$ 0.003 | 0.371 $\pm$ 0.006 | 0.036 $\pm$ 0.013 | 0.098 $\pm$ 0.034 |
| B-5   | True       | 0.168 $\pm$ 0.002 | 0.393 $\pm$ 0.005 | 0.029 $\pm$ 0.005 | 0.075 $\pm$ 0.012 |
| B-5   | False      | 0.162 $\pm$ 0.005 | 0.376 $\pm$ 0.010 | 0.037 $\pm$ 0.010 | 0.103 $\pm$ 0.027 |
| B-6   | True       | 0.160 $\pm$ 0.002 | 0.380 $\pm$ 0.006 | 0.030 $\pm$ 0.007 | 0.089 $\pm$ 0.017 |
| B-6   | False      | 0.160 $\pm$ 0.004 | 0.371 $\pm$ 0.006 | 0.028 $\pm$ 0.005 | 0.078 $\pm$ 0.015 |
| B-7   | True       | 0.157 $\pm$ 0.001 | 0.371 $\pm$ 0.005 | 0.026 $\pm$ 0.003 | 0.069 $\pm$ 0.007 |
| B-7   | False      | 0.159 $\pm$ 0.005 | 0.369 $\pm$ 0.010 | 0.036 $\pm$ 0.010 | 0.099 $\pm$ 0.027 |

Table 3. Detection performance for EfficientNet models with and without ImageNet pre-training at (384,384) pre-training and (384,480) fine-tuning resolution, evaluated on FLIR dataset’s in-domain (ID) and out-of-domain (OOD).

| Model | Pretrained | mAP-ID            | mAP50-ID          | mAP-OOD           | mAP50-OOD         |
|-------|------------|-------------------|-------------------|-------------------|-------------------|
| S     | True       | 0.202 $\pm$ 0.001 | 0.463 $\pm$ 0.002 | 0.059 $\pm$ 0.003 | 0.157 $\pm$ 0.006 |
| S     | False      | 0.184 $\pm$ 0.003 | 0.416 $\pm$ 0.002 | 0.043 $\pm$ 0.006 | 0.118 $\pm$ 0.014 |
| S-1   | True       | 0.181 $\pm$ 0.003 | 0.419 $\pm$ 0.004 | 0.055 $\pm$ 0.003 | 0.155 $\pm$ 0.014 |
| S-1   | False      | 0.177 $\pm$ 0.002 | 0.404 $\pm$ 0.007 | 0.039 $\pm$ 0.005 | 0.107 $\pm$ 0.015 |
| S-2   | True       | 0.172 $\pm$ 0.003 | 0.395 $\pm$ 0.005 | 0.047 $\pm$ 0.001 | 0.127 $\pm$ 0.002 |
| S-2   | False      | 0.174 $\pm$ 0.003 | 0.393 $\pm$ 0.006 | 0.036 $\pm$ 0.007 | 0.101 $\pm$ 0.024 |
| S-3   | True       | 0.156 $\pm$ 0.003 | 0.358 $\pm$ 0.004 | 0.023 $\pm$ 0.004 | 0.067 $\pm$ 0.009 |
| S-3   | False      | 0.163 $\pm$ 0.003 | 0.373 $\pm$ 0.008 | 0.036 $\pm$ 0.005 | 0.102 $\pm$ 0.013 |
| S-4   | True       | 0.150 $\pm$ 0.001 | 0.354 $\pm$ 0.004 | 0.031 $\pm$ 0.004 | 0.090 $\pm$ 0.012 |
| S-4   | False      | 0.150 $\pm$ 0.007 | 0.348 $\pm$ 0.014 | 0.040 $\pm$ 0.003 | 0.115 $\pm$ 0.007 |
| S-5   | True       | 0.141 $\pm$ 0.001 | 0.338 $\pm$ 0.004 | 0.022 $\pm$ 0.002 | 0.067 $\pm$ 0.007 |
| S-5   | False      | 0.141 $\pm$ 0.001 | 0.322 $\pm$ 0.004 | 0.035 $\pm$ 0.005 | 0.101 $\pm$ 0.014 |
| S-6   | True       | 0.136 $\pm$ 0.002 | 0.323 $\pm$ 0.004 | 0.023 $\pm$ 0.003 | 0.069 $\pm$ 0.005 |
| S-6   | False      | 0.140 $\pm$ 0.002 | 0.330 $\pm$ 0.005 | 0.023 $\pm$ 0.003 | 0.066 $\pm$ 0.007 |

Table 4. Detection performance for MobileNet models with and without ImageNet pre-training at (384,384) pre-training and (384,480) fine-tuning resolution, evaluated on FLIR dataset’s in-domain (ID) and out-of-domain (OOD).

| Model | Pretrained | mAP-ID | mAP50-ID | mAP-OOD | mAP50-OOD |
|-------|------------|--------|----------|---------|-----------|
| B-0   | True       | 0.663  | 0.899    | 0.592   | 0.804     |
| B-0   | False      | 0.643  | 0.895    | 0.585   | 0.812     |
| B-1   | True       | 0.651  | 0.903    | 0.598   | 0.822     |
| B-1   | False      | 0.650  | 0.908    | 0.589   | 0.810     |
| B-2   | True       | 0.552  | 0.864    | 0.506   | 0.758     |
| B-2   | False      | 0.545  | 0.850    | 0.486   | 0.730     |
| B-3   | True       | 0.499  | 0.825    | 0.454   | 0.712     |
| B-3   | False      | 0.535  | 0.850    | 0.513   | 0.788     |
| B-4   | True       | 0.459  | 0.809    | 0.406   | 0.677     |
| B-4   | False      | 0.490  | 0.797    | 0.449   | 0.697     |
| B-5   | True       | 0.448  | 0.776    | 0.386   | 0.626     |
| B-5   | False      | 0.508  | 0.843    | 0.468   | 0.725     |
| B-6   | True       | 0.467  | 0.791    | 0.453   | 0.730     |
| B-6   | False      | 0.505  | 0.823    | 0.489   | 0.754     |
| B-7   | True       | 0.476  | 0.819    | 0.472   | 0.747     |
| B-7   | False      | 0.526  | 0.838    | 0.511   | 0.777     |

Table 5. Detection performance for EfficientNet models with and without ImageNet pre-training at (384,384) pre-training and (256,192) fine-tuning resolution, evaluated on Distech dataset’s in-domain (ID) and out-of-domain (OOD).

| Model | Pretrained | mAP-ID | mAP50-ID | mAP-OOD | mAP50-OOD |
|-------|------------|--------|----------|---------|-----------|
| S     | True       | 0.603  | 0.891    | 0.555   | 0.809     |
| S     | False      | 0.586  | 0.883    | 0.560   | 0.820     |
| S-1   | True       | 0.572  | 0.876    | 0.543   | 0.807     |
| S-1   | False      | 0.565  | 0.864    | 0.514   | 0.762     |
| S-2   | True       | 0.568  | 0.870    | 0.502   | 0.749     |
| S-2   | False      | 0.562  | 0.865    | 0.528   | 0.780     |
| S-3   | True       | 0.552  | 0.863    | 0.513   | 0.771     |
| S-3   | False      | 0.553  | 0.869    | 0.470   | 0.715     |
| S-4   | True       | 0.512  | 0.843    | 0.461   | 0.723     |
| S-4   | False      | 0.498  | 0.812    | 0.471   | 0.731     |
| S-5   | True       | 0.492  | 0.825    | 0.486   | 0.761     |
| S-5   | False      | 0.503  | 0.826    | 0.455   | 0.716     |
| S-6   | True       | 0.496  | 0.820    | 0.457   | 0.708     |
| S-6   | False      | 0.498  | 0.820    | 0.486   | 0.750     |

Table 6. Detection performance for MobileNet models with and without ImageNet pre-training at (384,384) pre-training and (256,192) fine-tuning resolution, evaluated on Distech dataset’s in-domain (ID) and out-of-domain (OOD).
